# Supplementary material for: Parametrically driven Kerr cavity solitons
Source: arXiv:2101.07784 source file (2021-01-19)
Supplement: Supplementary file 1 [file SI.pdf]

# Parametrically driven Kerr cavity solitons

Nicolas Englebert,[1,*] Francesco De Lucia,[1,2] Pedro Parra-Rivas,[1] Carlos Mas Arabí,[1] Pier-John Sazio,[2] Simon-Pierre Gorza,[1] and François Leo[1]

[1]*Service OPERA-photonique, Université libre de Bruxelles (U.L.B.), 50 Avenue F. D. Roosevelt, CP 194/5, B-1050 Brussels, Belgium*

[2]*Optoelectronics Research Centre, University of Southampton, SO17 1BJ, United Kingdom*

This article contains the Supplementary Information for the manuscript entitled "Parametrically driven Kerr cavity solitons". We derive the parametrically driven nonlinear Schrödinger equation and perform a stability analysis of its stationary states. We also theoretically describe how parametric cavity solitons behave when the driving field is phase-modulated. Finally, additional experimental results are given.

## I. MEAN-FIELD MODEL

Pattern formation in our system can be described by a single mean-field equation at the signal frequency $\omega_0$. We here detail its derivation starting from the full lumped model. We start with a description of a passive singly resonant optical parametric oscillator incorporating a Kerr section. The cavity boundary conditions for both the signal field $A$ at $\omega_0$ and the pump field $B$ at $2\omega_0$ read [1]

$$A_{m+1}(0,\tau) = \sqrt{\mathcal{T}} A_m(L,\tau)\, \mathrm{e}^{i\varphi}, \quad \text{(S1)}$$

$$B_{m+1}(0,\tau) = B_{in}, \quad \text{(S2)}$$

where $m$ is the roundtrip number, $\mathcal{T} = \prod_k \mathcal{T}_k$ denotes the total insertion loss of all cavity components (polarization controllers, coupler, WDMs, ...) and $\varphi_0$ is the linear phase accumulated by the signal ($\omega_0$) over one roundtrip. The evolution of these fields in the periodically poled fibre (PPF) is given by the two following equations [2]

$$\frac{\partial A_m}{\partial z} = -\left(\frac{\alpha_s^{(1)}}{2} + i\frac{\beta_{2,s}^{(1)}}{2}\frac{\partial^2}{\partial \tau^2}\right) A_m + i\kappa B_m A_m^* \,\mathrm{e}^{-i\Delta\beta z}, \quad \text{(S3)}$$

$$\frac{\partial B_m}{\partial z} = -\left(\frac{\alpha_p^{(1)}}{2} + \Delta\beta_1^{(1)}\frac{\partial}{\partial \tau} + i\frac{\beta_{2,p}^{(1)}}{2}\frac{\partial^2}{\partial \tau^2}\right) A_m + i\kappa A_m^2 \,\mathrm{e}^{i\Delta\beta z}, \quad \text{(S4)}$$

where the subscript $s$ (resp. $p$) stands for signal (resp. pump). We introduce the superscript (1) for the parameters of the PPF. We will later use (2) for the SMF. For clarity, we drop the superscripts when defining the parameters in what follows. $z$ is the position along the fibre, $\tau = t - \beta_{1,s}z$ with $\beta_{1,s} = [\mathrm{d}\beta(\omega)/\mathrm{d}\omega]|_{\omega_0}$ where $\beta(\omega)$ is the propagation constant, $\Delta\beta = 2\beta(\omega_0) - \beta(2\omega_0)$ is the phase mismatch, $\Delta\beta_1 = \beta_{1,s} - \beta_{1,p}$ is the temporal walk-off where $\beta_{1,p} = [\mathrm{d}\beta(\omega)/\mathrm{d}\omega]|_{2\omega_0}$. $\beta_{2,s} = [\mathrm{d}^2\beta(\omega)/\mathrm{d}\omega^2]|_{\omega_0}$ and $\beta_{2,p} = [\mathrm{d}^2\beta(\omega)/\mathrm{d}\omega^2]|_{2\omega_0}$ are the group velocity dispersion coefficients. $\alpha_{s,p}$ are the loss coefficient and $\kappa$ is the second-order nonlinear parameter of the fibre. The third order nonlinearity is neglected because the PPF is much shorter than the total cavity length.

On the other hand, the signal evolution in the single-mode fibre (SMF) is described by the nonlinear Schrödinger equation (NLSE) [3]

$$\frac{\partial A_m}{\partial z} = -\left(\frac{\alpha_s^{(2)}}{2} + i\frac{\beta_{2,s}^{(2)}}{2}\frac{\partial^2}{\partial \tau^2} - i\gamma|A_m|^2\right) A_m, \quad \text{(S5)}$$

where $\gamma$ is the third-order nonlinear parameter of the fibre. The set of equations (S1)-(S5) constitute the full lumped model of the system. It is often referred to as a generalised Ikeda map [4]. This map can be reduced to a single mean-field equation following the approach described in [1, 2]. We consider that $A_m$ remains constant over one roundtrip and integrate (S4) over the length of the PPF. We find

$$B_m \approx B_{in}\,\mathrm{e}^{-\frac{\alpha_p^{(1)} z}{2}} + \kappa \int_{-\infty}^{\infty} \mathcal{F}[A_m^2] \frac{\mathrm{e}^{i\Delta\beta z} - \mathrm{e}^{\hat{k}z}}{\Delta\beta + i\hat{k}}\,\mathrm{e}^{-i\Omega\tau}\,\mathrm{d}\Omega, \quad \text{(S6)}$$

where $\mathcal{F}[\,\cdot\,]$ stands for the Fourier transform operator and $\hat{k} = -\alpha_p^{(1)}/2 + i(\Delta\beta_1\Omega + (\beta_{2,p}^{(1)}\Omega^2)/2)$. By substituting the latter expression in (S3) and integrating the result over the PPF length $L_1$ while keeping $A_m(z,\tau)$ constant, we find

$$\begin{aligned} A_m(L_1) \approx\; & A_m(0) - \left(\frac{\alpha_s^{(1)}}{2} + i\frac{\beta_{2,s}^{(1)}}{2}\frac{\partial^2}{\partial \tau^2}\right) L_1 A_m(0) \\ & + i\kappa B_{in}\,\mathrm{e}^{-i\xi}\frac{\sinh\xi}{\xi} L_1 A_m^*(0) \\ & - \rho^2\left[A_m^2 \otimes I(\tau)\right] A_m^*(0), \end{aligned} \quad \text{(S7)}$$

where $\xi = L_1(\alpha_p^{(1)} + i\Delta\beta)/2$, $\rho = \kappa L_1$, $I(\tau) = \mathcal{F}^{-1}[\hat{I}(\Omega)]$ is the kernel where $\mathcal{F}^{-1}[\,\cdot\,]$ stands for the inverse Fourier transform operator, $\hat{I}(\Omega) = (1 - ix - \mathrm{e}^{-ix})/x^2$ with $x(\Omega) = (\Delta\beta + i\hat{k})L_1$. The NLSE (S5) can also be integrated over the SMF length $L_2$, from $L_1$ to $L_1 + L_2 = L$

*Electronic address: nicolas.englebert@ulb.ac.be

while $A_m(z,\tau)$ is kept constant [5, 6]. We find

$$A_m(L) \approx A_m(L_1) - \left(\frac{\alpha_s^{(2)}}{2} + i\frac{\beta_{2,s}^{(2)}}{2}\frac{\partial^2}{\partial\tau^2} - i\gamma|A_m|^2\right) L_1 A_m. \tag{S8}$$

We substitute (S7) in (S8) and keep only the first order terms, obtaining

$$\begin{aligned} A_m(L) - A_m(0) \approx & -\left(\frac{\alpha_s^{(1)}}{2} + i\frac{\beta_{2,s}^{(1)}}{2}\frac{\partial^2}{\partial\tau^2}\right) L_1 A_m(0) \\ & + i\kappa B_{in}\,\mathrm{e}^{-i\xi}\,\frac{\sinh\xi}{\xi} L_1 A_m^*(0) \\ & -\rho^2\left[A_m^2 \otimes I(\tau)\right] A_m^*(0) \\ & -\left(\frac{\alpha_s^{(2)}}{2} + i\frac{\beta_{2,s}^{(2)}}{2}\frac{\partial^2}{\partial\tau^2} - i\gamma|A_m(0)|^2\right) L_2 A_m(0). \end{aligned} \tag{S9}$$

At first order, under the hypothesis of high finesse and by introducing the detuning $\delta_0 = 2k\pi - \varphi_0$ where $k$ is an integer, the boundary condition (S1) can be written

$$A_{m+1}(0) \approx \left(1 - \frac{\mathcal{R}}{2} - i\delta_0\right) A_m(L), \tag{S10}$$

where $\mathcal{R} = 1 - \mathcal{T}$. By substituting (S9) in (S10), we find the mean-field equation

$$\begin{aligned} t_R\frac{\partial A}{\partial T} = & \left(-\frac{\Lambda}{2} - i\delta_0 - i\frac{\underline{\beta_2 L}}{2}\frac{\partial^2}{\partial\tau^2} + i\gamma L_2|A|^2\right) A \\ & + \left(i\kappa B_{in} L_1 \mathrm{e}^{-\xi}\,\frac{\sinh\xi}{\xi} - \rho^2\left[A^2 \otimes I(\tau)\right]\right) A^*, \end{aligned} \tag{S11}$$

where we have introduced the slow-time $T = nt_R$ with $t_R$ the rountripe time, $\Lambda = \alpha_s^{(1)} L_1 + \alpha_s^{(2)} L_2 + \mathcal{R}$ and $\underline{\beta_2 L} = \beta_{2,s}^{(1)} L_1 + \beta_{2,s}^{(2)} L_2$. Equation (S11) describes pattern formation in a singly resonant optical parametric oscillator with a Kerr section. It is a generalisation of the model introduced in [1]. Next, we further generalise the model to account for an intracavity amplifier at the signal frequency. Equation (S11) becomes [7]:

$$\begin{aligned} t_R\frac{\partial A}{\partial T} = & \left(-\frac{\alpha}{2} + \frac{gL_3}{2} - i\delta_0 - i\frac{\underline{\beta_2 L}}{2}\frac{\partial^2}{\partial\tau^2} + i\gamma L_2|A|^2\right) A \\ & + \left(i\kappa B_{in} L_1 \mathrm{e}^{-\xi}\,\frac{\sinh\xi}{\xi} - \rho^2\left[A^2 \otimes I(\tau)\right]\right) A^*, \end{aligned} \tag{S12}$$

where $g$ is the gain per meter and $L_3$ the amplifier length. As the erbium ions relaxation time ($\tau_g = 10\,\mathrm{ms}$) is much longer than the roundtrip time ($t_R = 100\,\mathrm{ns}$) and providing that $t_R\langle|A(T,\tau)|^2\rangle \ll \tau_g P_{sat}$, the gain evolution over one roundtrip is given by [8, 9]

$$t_R\frac{\partial g}{\partial T} = -t_R\left(\frac{1}{\tau_g} + \frac{\langle|u(T,\tau)|^2\rangle}{\tau_g P_{sat}}\right) g + \frac{t_R g_0}{\tau_g}, \tag{S13}$$

where $\langle|u(T,\tau)|^2\rangle = \dfrac{1}{t_R}\displaystyle\int_0^{t_R} |u(T,\tau)|^2\,\mathrm{d}\tau$, $g_0$ is the unsaturated gain and and $P_{sat}$ is the saturation power. This equation and (S12) describe the dynamics of our system. Because the gain dynamics is slow in our case, we make the approximation $\partial_T g = 0$ which yields

$$g = \frac{g_0 L_3/2}{1 + \dfrac{\langle|u(T,\tau)|^2\rangle}{P_{sat}}}. \tag{S14}$$

In this paper, we focus on the detuning region ($0 < \delta_0 < 0.3$) where the intracavity filter does not impact the solitons. In that region, the average intracavity power $\langle|u(T,\tau)|^2\rangle$ is low and the gain stays close to its unsaturated value (i.e. $g \approx g_0$). The resonator intrinsic loss $\alpha$ can then be replaced by the effective loss $\Lambda_e$, defined as [9]

$$\Lambda_e = \Lambda - gL_3 \approx \Lambda - g_0 L_3. \tag{S15}$$

Moreover, the delayed third order term (describing upconversion) is also negligible in that region, leading to the following simplified mean-field equation, known as the parametrically driven nonlinear Schrödinger equation (PDNLSE) [10–12]

$$\begin{aligned} t_R\frac{\partial A}{\partial T} = & \left(-\frac{\Lambda_e}{2} - i\frac{\underline{\beta_2 L}}{2}\frac{\partial^2}{\partial\tau^2} - i\delta_0\right) A \\ & + \kappa B_{in} L_1 A^* + i\gamma L_2|A|^2 A \end{aligned} \tag{S16}$$

By introducing the parameters $T' = (\Lambda_e T)/t_R$, $\Delta = \delta_0/\Lambda_e$, $\tau' = \sqrt{\frac{2\Lambda_e}{|\underline{\beta_2 L}|}}$, $u = \sqrt{\frac{\gamma L_2}{\Lambda_e}} A$ and $\mu = \kappa B_{in} L_1/\Lambda_e$, we obtain the normalized, dimensionless version

$$\frac{\partial u}{\partial T'} = \left(-1 + i(|u|^2 - \Delta) + i\frac{\partial^2}{\partial\tau'^2}\right) u + \mu u^*. \tag{S17}$$

## II. LINEAR STABILITY ANALYSIS

To compute the linear stability of the homogeneous state solutions $u_h$ against generic perturbations $\xi(\tau,T)$, we first linearize the system around $u_h$ by introducing the ansatz $u(\tau,T) = u_h + \epsilon\xi(\tau,T) + c.c.$ ($|\epsilon| \ll 1$) in Eq. (S17). Keeping all the terms at first order in $\epsilon$, we obtain the linear equation

$$\partial_T \begin{bmatrix} \xi \\ \xi^* \end{bmatrix} = \begin{bmatrix} \mathsf{A} & \mathsf{B} \\ \mathsf{B}^* & \mathsf{A}^* \end{bmatrix} \begin{bmatrix} \xi \\ \xi^* \end{bmatrix}, \tag{S18}$$

where

$$\mathsf{A} \equiv -(1 + i\Delta) + i\partial_\tau^2 + 2i|u_h|^2, \quad \mathsf{B} \equiv iu_h^2 + \mu. \tag{S19}$$

To solve this equation, we consider modulated perturbation modes of the form $\xi(\tau,T) = a_\Omega e^{\sigma T + i\Omega\tau} + c.c.$, with $\Omega$

and $\sigma$ being the frequency and growth rate of the perturbation, respectively. This ansatz then leads to the linear system

$$\begin{bmatrix} \mathsf{A}_\Omega - \sigma & \mathsf{B} \\ \mathsf{B}^* & \mathsf{A}^*_\Omega - \sigma \end{bmatrix} \begin{bmatrix} a_\Omega \\ a^*_\Omega \end{bmatrix} = \begin{bmatrix} 0 \\ 0 \end{bmatrix}, \tag{S20}$$

with $\mathsf{A}_\Omega \equiv -(1+i\Delta) - i\Omega^2 + 2i|u_h|^2$, which has a non-trivial solution if

$$\sigma^2 + 2\sigma + f(\Omega) = 0, \qquad f(\Omega) = |\mathsf{A}_\Omega|^2 - |\mathsf{B}|^2, \tag{S21}$$

is satisfied. This condition yields to the dispersion relation

$$\sigma(\Omega) = -1 + \sqrt{1 - f(\Omega)}, \tag{S22}$$

which relates the growth of the perturbation $\xi$ with its frequency. If Re$[\sigma]$ is negative, the modulated perturbation $\xi$ decays, and $u_h$ is stable. However, when the contrary holds, the perturbation grows exponentially and $u_h$ is unstable. The transition occurs at the critical frequency $\Omega_c$ which satisfies simultaneously the conditions (i) $\sigma(\Omega)|_{\Omega_c} = 0$ and (ii) $\sigma'(\Omega)|_{\Omega_c} = 0$, with $(')$ denoting derivation with respect to $\Omega$.

### A. Stability of the trivial state

For the trivial state $u_h = 0$, $f(\Omega) = 1 - \mu^2 + (\Delta+\Omega^2)^2$, and the conditions (i)-(ii) lead respectively to

$$\mu^2 = 1 + (\Delta + \Omega_c^2)^2, \qquad (\Delta + \Omega_c^2)\Omega_c = 0, \tag{S23}$$

which define the onset of the instability and the critical frequency $\Omega_c$ of the growing perturbation at the instability. Depending on $\Omega_c$, two different instabilities take place. For $\Omega_c = 0$, a *pitchfork bifurcation*, occurs at $\mu = \mu_p \equiv \sqrt{1+\Delta^2}$, such that for $\mu < \mu_p$, $u_h = 0$ is stable against homogeneous perturbations and unstable otherwise. This instability corresponds to the degenerate OPO threshold.

In contrast, when $\Omega_c = \Omega_T \equiv \sqrt{-\Delta}$ and $\Delta < 0$, a *Turing or modulation instability* crops up at $\mu = \mu_T \equiv 1$, where $u_h = 0$ becomes unstable against modulated perturbations of frequency $\Omega_T$. This instability corresponds to the non-degenerate OPO threshold.

### B. Stability of the non-trivial state

The non-trivial homogeneous state can be written as $u_h = \sqrt{X}e^{i\phi}$, where $X$ satisfies $\mu^2 = 1 + (X - \Delta)^2$, and $\cos(2\phi) = \mu^{-1}$. For $\Delta > 0$, two non-trivial states $u_h^\pm$ exist, corresponding to the intensities $X^\pm \equiv \Delta \pm \sqrt{\mu^2 - 1}$. However, for $\Delta < 0$ the only nontrivial state corresponds to $u_h^+$ (i.e., to $X^+ \equiv \Delta + \sqrt{\mu^2-1}$).

In this case, $f = (2X - (\Delta + \Omega^2))^2 - \Delta^2$, and the dispersion relation reads [13]

$$\sigma^\pm = -1 + \sqrt{\Delta^2 + 1 - (\Delta \pm 2\sqrt{\mu^2-1} - \Omega^2)^2}. \tag{S24}$$

Here, the conditions (i)-(ii) become

$$X_c^\pm = \frac{1}{2}(\Omega_c^2 + \Delta \pm \Delta), \quad (\Delta + \Omega_c^2 - 2X)\Omega_c = 0. \tag{S25}$$

The condition $\Omega_c = 0$ leads to two instabilities. The first one occurs at $(\mu, X) = (\mu_p, 0)$ and corresponds to the *pitchfork bifurcation.* For $\Delta < 0$, $u_h^+$ bifurcates from $(\mu, u_h) = (\mu_p, 0)$ towards $\mu > \mu_p$, and the pitchfork bifurcation is called supercritical. In contrast, for $\Delta > 0$, $u_h^-$ bifurcates towards $\mu < \mu_p$, and the pitchfork bifurcation is subcritical. The second instability occurs at $(\mu, X) = (1, \Delta)$ for $\Delta > 0$, and corresponds to the *saddle-node bifurcation* SN$_h$ where $u_h^+$ and $u_h^-$ meet one another (i.e., $X^+ = X^-$).

For $\Omega_c \neq 0$, the conditions (i)-(ii) define the Turing instability, that in this case occurs at $\Delta = \Delta_T \equiv 0$ for a critical frequency $\Omega_T^2 = 2\sqrt{\mu^2-1}$. Below and above this line, the non-trivial state $u_h$ is modulationally unstable.

For $\Delta < 0$, $u_h^+$ is modulationally unstable, and the most unstable perturbation frequency is $\Omega_c^+ = \sqrt{\Delta + 2\sqrt{\mu^2-1}}$, which leads to $\sigma^+_{\rm max} = -1 + \sqrt{\Delta^2+1}$.

For $\Delta > 0$, $u_h^+$ preserves its modulationally unstable nature, and $u_h^-$ is modulationally unstable for $1 < \mu < \sqrt{\Delta^2/4+1}$, with a most unstable frequency $\Omega_c^- = \sqrt{\Delta - 2\sqrt{\mu^2-1}}$. In contrast, when $\sqrt{\Delta^2/4+1} < \mu < \mu_p$, the most unstable mode corresponds to $\Omega = 0$, therefore $u_h^-$ is unstable to homogeneous perturbations.

## III. PHASE MODULATION

Cavity solitons (CS) are known to be attracted to phase maxima of the driving beam [14]. In our experiment, we use a similar technique to lock the parametric cavity solitons (PCSs) on a 4.6 GHz grid. We imprint a periodic phase modulation $\phi(\tau)$ onto the driving laser prior to its frequency doubling. The resulting beam is phase modulated at twice the initial modulation frequency (see Fig. 3). Writing $\mu(\tau) = \mu_0 e^{i2\phi(\tau)}$, the mean-field equation (S17) becomes

$$\frac{\partial u}{\partial T} = \left(-1 + i(|u|^2 - \Delta) + i\frac{\partial^2}{\partial \tau^2}\right) u + \mu_0 e^{i2\phi(\tau)} u^*. \tag{S26}$$

By substituting $u = \bar{u}e^{i\phi(\tau)}$ into equation (S26), we find

$$\frac{\partial \bar{u}}{\partial T} = \Bigg( -(1+\phi'') + i(|\bar{u}|^2 - (\Delta + \phi'^2)) + i\frac{\partial^2}{\partial \tau^2} - 2\phi'\frac{\partial}{\partial \tau}\Bigg)\bar{u} + \mu_0 \bar{u}^*, \tag{S27}$$

where $\phi' = \frac{d\phi}{d\tau}$ and $\phi'' = \frac{d^2\phi}{d\tau^2}$. The impact of $\phi''$ (resp. $\phi'^2$) over the total losses (resp. detuning) is small [14]. The term $2\phi'\partial_\tau$ provides a local $\tau$-dependent variation of

the group velocity. When $\phi' > 0$ (resp. $\phi' < 0$), the soliton suffers a delay (resp. advancement) with respect to the carrier frequency reference frame. This implies that individual PCS will lock to a phase modulation maximum.

## References


1. Mosca, S. *et al.* Modulation Instability Induced Frequency Comb Generation in a Continuously Pumped Optical Parametric Oscillator. *Physical Review Letters* **121,** 093903 (2018).
2. Leo, F. *et al.* Walk-Off-Induced Modulation Instability, Temporal Pattern Formation, and Frequency Comb Generation in Cavity-Enhanced Second-Harmonic Generation. *Physical Review Letters* **116,** 033901 (2016).
3. Agrawal, G. *Nonlinear Fiber Optics* (Academic Press, 2013).
4. Ikeda, K. Multiple-valued stationary state and its instability of the transmitted light by a ring cavity system. *Optics Communications* **30,** 257–261 (1979).
5. Lugiato, L. A. & Lefever, R. Spatial Dissipative Structures in Passive Optical Systems. *Physical Review Letters* **58,** 2209–2211 (1987).
6. Haelterman, M., Trillo, S. & Wabnitz, S. Dissipative modulation instability in a nonlinear dispersive ring cavity. *Optics Communications* **91,** 401–407 (1992).
7. Komarov, A., Leblond, H. & Sanchez, F. Multistability and hysteresis phenomena in passively mode-locked fiber lasers. *Physical Review A* **71,** 053809 (2005).
8. Haboucha, A., Leblond, H., Salhi, M., Komarov, A. & Sanchez, F. Analysis of soliton pattern formation in passively mode-locked fiber lasers. *Physical Review A* **78,** 043806 (2008).
9. Englebert, N., Gorza, S.-P. & Leo, F. Temporal Solitons in a Coherently Driven Active Resonator. *arXiv:2007.15630 [physics]* (2020).
10. Miles, J. W. Parametrically excited solitary waves. fr. *Journal of Fluid Mechanics* **148,** 451–460 (1984).
11. Denardo, B. *et al.* Observations of localized structures in nonlinear lattices: Domain walls and kinks. *Physical Review Letters* **68,** 1730–1733 (1992).
12. Longhi, S. Ultrashort-pulse generation in degenerate optical parametric oscillators. *Optics Letters* **20,** 695–697 (1995).
13. Longhi, S. & Geraci, A. Modulational instability oscillation and solitary waves in a nonlinear dispersive cavity with parametric gain. *Applied Physics Letters* **67,** 3060–3062 (1995).
14. Jang, J. K., Erkintalo, M., Coen, S. & Murdoch, S. G. Temporal tweezing of light through the trapping and manipulation of temporal cavity solitons. *Nature Communications* **6,** 7370 (2015).

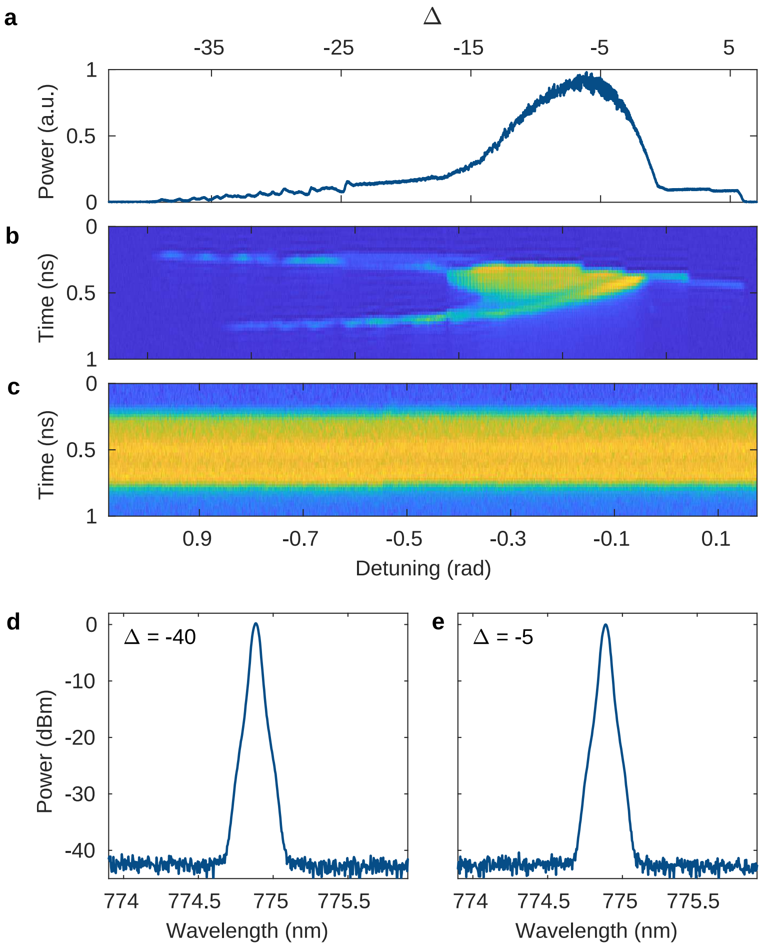


**Fig. S1. Spontaneous Parametric Cavity Solitons generation.** **a**, Cavity resonance measured with a 200 kHz photodiode. The scan leads to the generation of a multiple soliton-step, i.e. the spontaneous generation of multiple PCSs. **b**, Similar scan performed with a 12 GHz detection system. The oscillation is initiated on the edges of the driving pulse, after which the signal broadens to reach the same duration as the pump pulse and eventually collapses on the soliton state. **c**, Corresponding pump pulse profile. It remains unchanged throughout the scan which validates the constant pump approximation used in our model. **d**, Pump spectrum below and above (**e**) the oscillation threshold. The absence of spectral broadening further confirms that cascaded nonlinearites do not play a significant role in our system.
